# Supplementary material for: An AMM minimizing user-level extractable value and loss-versus-rebalancing
Source: arXiv:2301.13599 source file (2023-02-15)
Supplement: Supplementary file 1 [file Proofs.tex]

\input{Appendices/RelatedWork}
